# Supplementary material for: Centralized Defense: Logging and Mitigation of Kubernetes Misconfigurations with Open Source Tools
Source: arXiv:2408.03714 source file (2024-08-07)
Supplement: Supplementary file 1 [file AppendixA.tex]

\chapter{Code Snippets}

\lstset{
	language=bash,
	basicstyle=\footnotesize\ttfamily,
	breaklines=true, % enables line breaking
	postbreak=\mbox{\textcolor{red}{$\hookrightarrow$}\space}, % marks where line was broken
	frame=single, % adds a frame around the code
	numbers=left, % line numbers on left
	numberstyle=\tiny\color{gray}, % line numbers styling
	showstringspaces=false, % don't show spaces in strings as special character
	tabsize=3, % sets tab size to 3 spaces
	captionpos=b % sets the caption position to bottom
}

\section{Download Tools Script}

\begin{lstlisting}[language=bash, caption={Download tools Script}, basicstyle=\footnotesize\ttfamily, label={lst:download_tools_script}]
	#!/bin/bash
	
	# Define the tool names and their corresponding release URLs
	TOOLS=(
	"trivy|https://github.com/aquasecurity/trivy/releases/latest"
	"kubesec|https://github.com/controlplaneio/kubesec/releases/latest"
	"kube-linter|https://github.com/stackrox/kube-linter/releases/latest"
	"kube-score|https://github.com/zegl/kube-score/releases/latest"
	)
	
	DOWNLOAD_URLS=(
	"trivy|https://github.com/aquasecurity/trivy/releases/download/vversion/trivy_version_Linux-64bit.tar.gz"
	"kubesec|https://github.com/controlplaneio/kubesec/releases/download/vversion/kubesec_linux_arm64.tar.gz"
	"kube-linter|https://github.com/stackrox/kube-linter/releases/download/vversion/kube-linter-linux.tar.gz"
	"kube-score|https://github.com/zegl/kube-score/releases/download/vversion/kube-score_version_linux_amd64.tar.gz"
	)
	
	INSTALL_DIR="bin"
	mkdir -p $INSTALL_DIR
	
	# Function to get the latest version of a tool
	get_latest_version() {
		local tool_info="$1"
		local releases_url=$(echo $tool_info | cut -d '|' -f 2)
		
		local release_url=$(curl -sSLI -o /dev/null -w '%{url_effective}' $releases_url)
		local version=$(basename $release_url | sed 's/^v//')
		
		echo "$version"
	}
	
	# Loop through the array of tools and get the latest versions
	for tool_info in "${TOOLS[@]}"; do
	version=$(get_latest_version "$tool_info")
	tool_name=$(echo $tool_info | cut -d '|' -f 1)
	
	echo "Downloading $tool_name version $version..."
	
	# Find the corresponding download URL for the current tool
	for download_url_info in "${DOWNLOAD_URLS[@]}"; do
	download_tool_name=$(echo "$download_url_info" | cut -d '|' -f 1)
	tool_url=$(echo "$download_url_info" | cut -d '|' -f 2)
	
	# Check if the tool names match
	if [ "$download_tool_name" == "$tool_name" ]; then
	# Construct the download URL using the version
	download_url=$(echo "$tool_url" | sed "s/version/$version/g")
	echo $version
	
	# Download the tool
	if [[ $download_url == *.tar.gz ]]; then
	wget "$download_url" -O "$INSTALL_DIR/$download_tool_name-$version.tar.gz"
	tar -xvzf $INSTALL_DIR/$download_tool_name-$version.tar.gz -C $INSTALL_DIR $tool_name
	rm $INSTALL_DIR/$download_tool_name-$version.tar.gz
	elif [[ $download_url == *.zip ]]; then
	wget "$download_url" -O "$INSTALL_DIR/$download_tool_name-$version.zip"
	unzip -j $INSTALL_DIR/$download_tool_name-$version.zip -d $INSTALL_DIR *$tool_name
	rm $INSTALL_DIR/$download_tool_name-$version.tar.gz
	fi
	echo "Download complete!"
	fi
	done
	done
\end{lstlisting}

\section{Run Script}

\begin{lstlisting}[caption={Security Analysis Script}, label={lst:security_analysis_script}]
#!/bin/bash

output_dir="/output"
manifest_dir="$output_dir/manifest"
kubesec_dir="$output_dir/kubesec"
trivy_dir="$output_dir/trivy"
kube_score_dir="$output_dir/kube-score"
kube_linter_dir="$output_dir/kube-linter"


script_dir="$(cd "$(dirname "${BASH_SOURCE[0]}")" && pwd)"
bin_dir="$script_dir/bin"
kubesec_path="$bin_dir/kubesec"
trivy_path="$bin_dir/trivy"
kube_score_path="$bin_dir/kube-score"
kube_linter_path="$bin_dir/kube-linter"  

# Create the output directories if they don't exist
mkdir -p "$manifest_dir"
mkdir -p "$kubesec_dir"
mkdir -p "$trivy_dir"
mkdir -p "$kube_score_dir"
mkdir -p "$kube_linter_dir" 

# List all namespaces
namespaces=$(kubectl get namespaces -o jsonpath='{.items[*].metadata.name}')

# Iterate through namespaces
for namespace in $namespaces; do
    # List all pods in the namespace
    pods=$(kubectl get pods -n $namespace -o jsonpath='{.items[*].metadata.name}')

    # Iterate through pods
    for pod in $pods; do
        # Get pod manifest
        manifest_file="$manifest_dir/$pod-manifest.yaml"
        kubectl get pod $pod -n $namespace -o yaml > "$manifest_file"

        # Run kubesec
        "$kubesec_path" scan "$manifest_file" --output json | \
        jq '.[].scoring.advise | map({
        id: .id, 
        selector: .selector, 
        reason: .reason, 
        points: .points, 
        severity: (
            if .points == -30 then "CRITICAL"
            elif .points == -9 or .points == -7 then "HIGH"
            elif .points == -3 or .points == -1 then "MEDIUM"
            elif .points == 1 or .points == 3 then "LOW"
            else "UNKNOWN" 
            end
        )
        })' > "$kubesec_dir/$pod-result.json"

        # Run trivy
       "$trivy_path" fs --scanners vuln,secret,misconfig "$manifest_file" -f json --output $trivy_dir/$pod-result.json
        jq -r '.Results[] | .Misconfigurations[] | if type == "object" then { Type: .Type, ID: .ID, AVDID: .AVDID, Title: .Title, Description: .Description, Message: .Message, Resolution: .Resolution, Severity: .Severity } else empty end' "$trivy_dir/$pod-result.json" | \
        jq -s 'map(select(.Severity)) | sort_by({ "CRITICAL": -3, "HIGH": -2, "MEDIUM": -1, "LOW": 0 }[.Severity])' > "$trivy_dir/$pod-result-updated.json"
        echo "moving file"
        mv "$trivy_dir/$pod-result-updated.json" "$trivy_dir/$pod-result.json"

        # Run kube-score
        #"$kube_score_path" score "$manifest_file" --output-format json | \
        #jq '[.[] | .checks[] | {name: .check.name, id: .check.id, comment: .check.comment, grade: .grade, severity: (if .grade == 10 then "CRITICAL" elif .grade >= 7 and .grade < 10 then "HIGH" elif .grade >= 5 and .grade < 7 then "MEDIUM" else "LOW" end)}]' > "$kube_score_dir/$pod-result.json"
        "$kube_score_path" score "$manifest_file" --output-format json | \
        jq '[.[] | .checks[] | {
        name: .check.name,
        id: .check.id,
        comment: .check.comment,
        grade: .grade,
        severity: (
            if .grade == 10 then "CRITICAL"
            elif .grade >= 7 and .grade < 10 then "HIGH"
            elif .grade >= 5 and .grade < 7 then "MEDIUM"
            elif .grade < 5 then "LOW"
            else "UNKNOWN"
            end
        )
        }]' > "$kube_score_dir/$pod-result.json"


        # Run kube-linter
        "$kube_linter_path" lint "$manifest_file" --format json | \
        jq '.Reports | map({Check: .Check, Message: .Diagnostic.Message, Remediation: .Remediation, Severity: "Unknown"})' > "$kube_linter_dir/$pod-result.json"
    
 done
done
\end{lstlisting}

\section{Compare Python Script}

\lstset{
    language=Python,
    basicstyle=\footnotesize\ttfamily,
    breaklines=true,
    frame=single,
    postbreak=\mbox{\textcolor{red}{$\hookrightarrow$}\space},
    showstringspaces=false,
    numbers=left,
    numberstyle=\tiny\color{gray},
    keywordstyle=\color{blue},
    commentstyle=\color{green}
}

\begin{lstlisting}[caption={Python Script to compare tool outputs}, label={lst:python_script}]
import json
import os
from difflib import SequenceMatcher

def find_similar_issues(trivy_output, kubesec_file_path, kubesec_output, kubescore_output, kubelint_output):

    # Finds similar issues between outputs.
    trivy_issues = []
    kubesec_issues = []
    kubescore_issues = []
    kubelint_issues = []
    
    for item in trivy_output:
        trivy_issues.append(item)

    for item in kubesec_output:
        kubesec_issues.append(item)

    for item in kubescore_output:
        kubescore_issues.append(item)
    
    for item in kubelint_output:
        kubelint_issues.append(item)
        
    for trivy_issue in trivy_issues:
        for kubesec_issue in kubesec_issues:
            similarity_score = SequenceMatcher(None, trivy_issue['Resolution'], kubesec_issue['selector']).ratio()
            if similarity_score >= 0.65:
                kubesec_issues.remove(kubesec_issue)
                break 
    
    with open(kubesec_file_path, 'w') as kubesec_json_file:
        json.dump(kubesec_issues, kubesec_json_file, indent=4)

trivy_dir = '/output/trivy'
kubesec_dir = '/output/kubesec'
kubescore_dir = '/output/kube-score'
kubelint_dir = '/output/kube-linter'

# Get the list of files in each directory
trivy_files = set(os.listdir(trivy_dir))
kubesec_files = set(os.listdir(kubesec_dir))
kubescore_files = set(os.listdir(kubescore_dir))
kubelink_files = set(os.listdir(kubelint_dir))

# Find common file names
common_files = trivy_files.intersection(kubesec_files)

# Iterate through common file names and compare corresponding files
for file_name in common_files:
    print("Comparing file:", file_name)
    trivy_file_path = os.path.join(trivy_dir, file_name)
    kubesec_file_path = os.path.join(kubesec_dir, file_name)
    kubescore_file_path = os.path.join(kubescore_dir, file_name)
    kubelint_file_path = os.path.join(kubelint_dir, file_name)

    with open(trivy_file_path, 'r') as trivy_file:
        trivy_output = json.load(trivy_file)

    with open(kubesec_file_path, 'r') as kubesec_file:
        kubesec_output = json.load(kubesec_file)

    with open(kubescore_file_path, 'r') as kubescore_file:
        kubescore_output = json.load(kubescore_file)

    with open(kubelint_file_path, 'r') as kubelint_file:
        kubelint_output = json.load(kubelint_file)
    
    # Call the function to find similar issues
    find_similar_issues(trivy_output, kubesec_file_path, kubesec_output, kubescore_output, kubelint_output)
\end{lstlisting}

\section{Convert outputs to common template}

\begin{lstlisting}[caption={Convert json outputs to a common template}, label={lst:json_conversion}]
#!/bin/bash

# Define the directory containing the JSON files
kubesec_dir="/output/kubesec"
kubescore_dir="/output/kube-score"
kubelint_dir="/output/kube-linter"

# Iterate over each JSON file in the directory
for file_path in "$kubesec_dir"/*.json; do
    # Apply jq transformation and override the file
    jq 'map(
        {
            "Type": "Kubernetes Security Check",
            "ID": "",
            "AVDID": "",
            "Title": .id,
            "Description": "",
            "Message": .reason,
            "Resolution": .selector,
            "Severity": .severity
        }
    )' "$file_path" > "$file_path.tmp" && mv "$file_path.tmp" "$file_path"
done

for file_path in "$kubescore_dir"/*.json; do
    # Apply jq transformation and override the file
    jq 'map(
        {
            "Type": "Kubernetes Security Check",
            "ID": .id,
            "AVDID": "",
            "Title": .name,
            "Description": "",
            "Message": .comment,
            "Resolution": "",
            "Severity": .severity
        }
    )' "$file_path" > "$file_path.tmp" && mv "$file_path.tmp" "$file_path"
done

for file_path in "$kubelint_dir"/*.json; do
    # Apply jq transformation and override the file
    jq 'map(
        {
            "Type": "Kubernetes Security Check",
            "ID": "",
            "AVDID": "",
            "Title": .Check,
            "Description": "",
            "Message": .Message,
            "Resolution": .Remediation,
            "Severity": .Severity
        }
    )' "$file_path" > "$file_path.tmp" && mv "$file_path.tmp" "$file_path"
done
\end{lstlisting}

\section{Merge JSON files}

\begin{lstlisting}[caption={Merging JSON Outputs}, label={lst:json_merging_bash_script}]
#!/bin/bash

trivy_dir="/output/trivy"
kubesec_dir="/output/kubesec"
kubescore_dir="/output/kube-score"
kubelint_dir="/output/kube-linter"
output_dir="/output/merged"

# Create the output directory if it doesn't exist
mkdir -p "$output_dir"

# Get the list of files in the trivy directory
trivy_files=$(cd "$trivy_dir" && ls *.json)

# Iterate over each trivy file
for trivy_file in $trivy_files; do
    # Initialize an array to hold the files to merge
    files_to_merge=("$trivy_dir/$trivy_file")

    # Check if there is a matching file in kubesec directory
    if [ -f "$kubesec_dir/$trivy_file" ]; then
        files_to_merge+=("$kubesec_dir/$trivy_file")
    fi

    # Check if there is a matching file in kube-score directory
    if [ -f "$kubescore_dir/$trivy_file" ]; then
        files_to_merge+=("$kubescore_dir/$trivy_file")
    fi

    # Check if there is a matching file in kube-linter directory
    if [ -f "$kubelint_dir/$trivy_file" ]; then
        files_to_merge+=("$kubelint_dir/$trivy_file")
    fi

    # Merge contents of all found files
    jq -s 'flatten' "${files_to_merge[@]}" > "$output_dir/$trivy_file"
done
\end{lstlisting}

\section{Send data to mongodb}

\begin{lstlisting}[caption={Send data to MongoDB}, label={lst:python_mongodb}]
import os
import json
from pymongo import MongoClient

client = MongoClient('mongodb://mongo-service:27017/')
db = client['json_database']

root_directory = '/output/merged/'
json_files = []

# Traverse through the directory structure to find JSON files
for dirpath, dirnames, filenames in os.walk(root_directory):
    for filename in filenames:
        if filename.endswith('.json'):
            json_files.append(os.path.join(dirpath, filename))

# Iterate over each JSON file
for file_path in json_files:
    with open(file_path) as file:
        try:
            # Load JSON data from the file
            json_data = json.load(file)
            
            # Extract collection name from the file name
            collection_name = os.path.splitext(os.path.basename(file_path))[0]
            
            # Get the collection in the MongoDB database
            collection = db[collection_name]
            
            collection.delete_many({})
            
            # Insert each JSON object into the collection
            for item in json_data:
                collection.insert_one(item)
            
            print(f"Inserted data from {file_path} into collection {collection_name}")
        except Exception as e:
            print(f"Error inserting data from {file_path} into MongoDB: {e}")
\end{lstlisting}

\section{Flask app}

\begin{lstlisting}[caption={Flask App}, label={lst:flask_app}]
from flask import Flask, render_template
from flask_pymongo import PyMongo

app = Flask(__name__)
app.config["MONGO_URI"] = "mongodb://mongo-service:27017/json_database"
mongo = PyMongo(app)

# Set the Flask port to 5002
app.config['FLASK_RUN_PORT'] = 5002

@app.route('/')
def index():
    collections = mongo.db.list_collection_names()
    vulnerabilities = {}
    collection_vulnerabilities = {}  # Corrected initialization placement
    for collection_name in collections:
        collection = mongo.db[collection_name]
        documents = collection.find()
        collection_vulnerabilities[collection_name] = {}  # Initialize the inner dictionary for each collection
        for document in documents:
            severity = document.get('Severity', 'Unknown')
            if severity in vulnerabilities:
                vulnerabilities[severity] += 1
            else:
                vulnerabilities[severity] = 1
                
            if severity in collection_vulnerabilities[collection_name]:
                collection_vulnerabilities[collection_name][severity] += 1
            else:
                collection_vulnerabilities[collection_name][severity] = 1

    return render_template('index.html', vulnerabilities=vulnerabilities, collection_vulnerabilities=collection_vulnerabilities)

@app.route('/vulnerabilities/<severity>')
def show_vulnerabilities(severity):
    collections = mongo.db.list_collection_names()
    vulnerabilities = []
    for collection_name in collections:
        collection = mongo.db[collection_name]
        documents = collection.find({'Severity': severity})
        for document in documents:
            document['collection_name'] = collection_name  
            vulnerabilities.append(document)
    return render_template('vulnerabilities.html', severity=severity, vulnerabilities=vulnerabilities)

@app.route('/collection/<collection_name>')
def show_collection_vulnerabilities(collection_name):
    vulnerabilities = []
    collection = mongo.db[collection_name]
    documents = collection.find()
    for document in documents:
        vulnerabilities.append(document)
    return render_template('collection_vulnerabilities.html', collection_name=collection_name, vulnerabilities=vulnerabilities)

if __name__ == '__main__':
    app.run(debug=True)
\end{lstlisting}

\section{HTML Templates}

\lstset{
    language=HTML,
    basicstyle=\footnotesize\ttfamily,
    breaklines=true,
    frame=single,
    postbreak=\mbox{\textcolor{red}{$\hookrightarrow$}\space},
    showstringspaces=false,
    numbers=left,
    numberstyle=\tiny\color{gray},
    keywordstyle=\color{blue},
    commentstyle=\color{green}
}

\subsection{Current Vulnerabilities Template}
\begin{lstlisting}[caption={Current Vulnerabilities HTML Template}]
<!DOCTYPE html>
<html lang="en">
<head>
    <meta charset="UTF-8">
    <meta name="viewport" content="width=device-width, initial-scale=1.0">
    <title>Current Vulnerabilities</title>
    <style>
        table {
            width: 50%;
            border-collapse: collapse;
        }
        th, td {
            border: 1px solid #dddddd;
            text-align: left;
            padding: 8px;
        }
        th {
            background-color: #f2f2f2;
        }
        .top-bar {
            background-color: #f2f2f2;
            padding: 10px;
            margin-bottom: 10px;
            overflow: hidden;
        }
        #refresh-popup {
            position: fixed;
            top: 0;
            left: 50%;
            transform: translateX(-50%);
            width: 200px;
            background-color: #ccc;
            color: #333;
            text-align: center;
            padding: 10px;
            display: none;
            z-index: 999;
        }
    </style>
    <script>
        function autoRefresh() {
            showRefreshPopup();
            setTimeout(function () {
                location.reload();
            }, 30000);
        }

        function showRefreshPopup() {
            var popup = document.getElementById("refresh-popup");
            popup.style.display = "block";
            setTimeout(function() {
                popup.style.display = "none";
            }, 2000);
        }

        window.onload = autoRefresh;
        window.addEventListener('pageshow', function(event) {
            autoRefresh();
        });
    </script>
</head>
<body>
    <div id="refresh-popup">Refreshing...</div>
    <div class="top-bar">
        <h2>Current Vulnerabilities</h2>
    </div>
    <table>
        <thead>
            <tr>
                <th>Severity</th>
                <th>Number of Vulnerabilities</th>
            </tr>
        </thead>
        <tbody>
            {% for severity, count in vulnerabilities.items() %}
            <tr>
                <td><a href="/vulnerabilities/{{ severity }}">{{ severity }}</a></td>
                <td>{{ count }}</td>
            </tr>
            {% endfor %}
        </tbody>
    </table>
    <h2>Collection-wise Vulnerabilities</h2>
    <table>
        <thead>
            <tr>
                <th>Collection Name</th>
                <th>High</th>
                <th>Medium</th>
                <th>Low</th>
            </tr>
        </thead>
        <tbody>
            {% for collection, severities in collection_vulnerabilities.items() %}
            <tr>
                <td><a href="/collection/{{ collection }}">{{ collection }}</a></td>
                <td>{{ severities.get('HIGH', 0) }}</td>
                <td>{{ severities.get('MEDIUM', 0) }}</td>
                <td>{{ severities.get('LOW', 0) }}</td>
            </tr>
            {% else %}
            <tr>
                <td><a href="/collection/{{ collection }}">{{ collection }}</a></td>
                <td>0</td>
                <td>0</td>
                <td>0</td>
            </tr>
            {% endfor %}
        </tbody>
    </table>
</body>
</html>
\end{lstlisting}

\subsection{Vulnerabilities by Severity Template}
\begin{lstlisting}[caption={Vulnerabilities by Severity HTML Template}]
<!DOCTYPE html>
<html lang="en">
<head>
    <meta charset="UTF-8">
    <meta name="viewport" content="width=device-width, initial-scale=1.0">
    <title>{{ severity }} Vulnerabilities</title>
    <style>
        table {
            width: 100%;
            border-collapse: collapse;
        }
        th, td {
            border: 1px solid #dddddd;
            text-align: left;
            padding: 8px;
        }
        th {
            background-color: #f2f2f2;
        }
        .top-bar, .back-button {
            background-color: #f2f2f2;
            padding: 10px;
            margin-bottom: 10px;
            overflow: hidden;
            float: left;
            margin-right: 10px;
        }
        #refresh-popup {
            position: fixed;
            top: 0;
            left: 50%;
            transform: translateX(-50%);
            width: 200px;
            background-color: #ccc;
            color: #333;
            text-align: center;
            padding: 10px;
            display: none;
            z-index: 999;
        }
    </style>
    <script>
        function autoRefresh() {
            showRefreshPopup();
            setTimeout(function () {
                location.reload();
            }, 30000);
        }

        function showRefreshPopup() {
            var popup = document.getElementById("refresh-popup");
            popup.style.display = "block";
            setTimeout(function() {
                popup.style.display = "none";
            }, 2000);
        }

        function goBack() {
            window.history.back();
        }

        window.onload = autoRefresh;
        window.addEventListener('pageshow', function(event) {
            autoRefresh();
        });
    </script>
</head>
<body>
    <div id="refresh-popup">Refreshing...</div>
    <div class="top-bar">
        <button class="back-button" onclick="goBack()">Back</button>
        <h2>{{ severity }} Vulnerabilities</h2>
    </div>
    <table>
        <thead>
            <tr>
                <th>Collection Name</th>
                <th>Severity</th>
                <th>Title</th>
                <th>AVDID</th>
                <th>Description</th>
                <th>Message</th>
                <th>Resolution</th>
            </tr>
        </thead>
        <tbody>
            {% for document in vulnerabilities %}
            <tr>
                <td>{{ document.collection_name }}</td>
                <td>{{ document.Severity }}</td>
                <td>{{ document.Title }}</td>
                <td>{{ document.AVDID }}</td>
                <td>{{ document.Description }}</td>
                <td>{{ document.Message }}</td>
                <td>{{ document.Resolution }}</td>
            </tr>
            {% endfor %}
        </tbody>
    </table>
</body>
</html>
\end{lstlisting}

\subsection{JSON Data Overview Template}
\begin{lstlisting}[caption={JSON Data Overview HTML Template}]
<!DOCTYPE html>
<html>
<head>
    <title>JSON Data</title>
    <style>
        table {
            width: 100%;
            border-collapse: collapse;
            margin-bottom: 20px;
        }
        th, td {
            padding: 8px;
            text-align: left;
            border-bottom: 1px solid #ddd;
        }
        th {
            background-color: #f2f2f2;
        }
    </style>
</head>
<body>
    {% for collection_name, documents in collection_data.items() %}
    <h2>{{ collection_name }}</h2>
    <table>
        <tr>
            <th>AVDID</th>
            <th>Description</th>
            <th>ID</th>
            <th>Message</th>
            <th>Resolution</th>
            <th>Severity</th>
            <th>Title</th>
            <th>Type</th>
        </tr>
        {% for document in documents %}
        <tr>
            <td>{{ document.AVDID }}</td>
            <td>{{ document.Description }}</td>
            <td>{{ document.ID }}</td>
            <td>{{ document.Message }}</td>
            <td>{{ document.Resolution }}</td>
            <td>{{ document.Severity }}</td>
            <td>{{ document.Title }}</td>
            <td>{{ document.Type }}</td>
        </tr>
        {% endfor %}
    </table>
    {% endfor %}
</body>
</html>
\end{lstlisting}
